# Supplementary material for: A Multi-objective Evolutionary Algorithm Based on Bi-population with Uniform Sampling for Neural Architecture Search
Source: arXiv:2602.08513 source file (2026-02-09)
Supplement: Supplementary file 1 [file SupplementaryMaterial.pdf]

**Supplementary Material**

# A Multi-objective Evolutionary Algorithm Based on Bi-population with Uniform Sampling for Neural Architecture Search

Yu Xue, *Senior Member, IEEE*, Pengcheng Jiang, *Graduate Student Member, IEEE*, Chenchen Zhu, Yong Zhang, *Senior Member, IEEE*, Ran Cheng, *Senior Member, IEEE*, Kaizhou Gao, *Senior Member, IEEE*, Dunwei Gong, *Senior Member, IEEE*

***Abstract*—This is the supplementary material for the paper titled "A Multi-objective Evolutionary Algorithm Based on Bi-population with Uniform Sampling for Neural Architecture Search". Section I reports the comparison search results on the CIFAR-100 dataset, including accuracy, the number of parameters, MAdds and search cost. Section II reports an ablation study on surrogate model performance, using visualization methods to present the effects of different surrogate modes (regression prediction and pairwise comparison relationship prediction), initialization methods, and base machine learning models on surrogate performance. Section III reports the surrogate time costs for different base machine learning models using both regression prediction and pairwise comparison relationship prediction.**

***Index Terms*—Evolutionary algorithm, neural architecture search, multi-objective optimization, multi-population mechanism, surrogate model.**

## I. Search Results on CIFAR-100

CIFAR-100 is a standard dataset widely used for neural architecture search (NAS) comparison, along with CIFAR-10 and ImageNet. Similar to CIFAR-10, CIFAR-100 also contains 60,000 images with a size of 32 $\times$ 32 pixels. The difference is that CIFAR-100 has 100 categories, thereby increasing the difficulty of classification.

Similar to the experimental setting on CIFAR-10, we also conduct experiments on CIFAR-100. Table I presents the experimental results of MOEA-BUS on CIFAR-100 and compares them with other NAS methods. The results show that the MOEA-BUS method performs well in balancing accuracy and MAdds, and has a significant advantage in search time compared to some other methods. In terms of accuracy, MOEA-BUS shows excellent performance. The accuracy of different sized MOEA-BUS models (MOEA-BUS-S/M/L/XL) all exceed 86%, with MOEA-BUS-XL achieving the highest accuracy of 88.01%. This surpasses most existing NAS methods, especially the multi-objective ENAS and multi-population ENAS [11], [15], [16], and is significantly better than GD-based algorithms like the DARTS series, which usually have lower accuracies of around 83% to 84%. Regarding model complexity, the MAdds values of the architectures found by our method are relatively low. MOEA-BUS-S has a MAdds of 198M, while the largest MOEA-BUS-XL is 657M. These complexity values are much lower than those of NASNet-A [3] series models, such as NASNet-A Large, which has a MAdds of up to 12031M. Although there are certain differences in MAdds values for MOEA-BUS, it maintains a relatively moderate computational complexity while ensuring high accuracy, making it highly scalable and computationally efficient in practical applications. In terms of search time, the MOEA-BUS method also has a significant advantage. It takes only 1.2 GPU days to search, while other methods like FairNAS series need 12 GPU days. Compared to FX-DARTS [10], the obtained MOEA-BUS-S can achieve an approximately 8.7% classification accuracy advantage, while the MAdds remains nearly consistent with FX-DARTS. Compared to SPNAS [18], which also uses the MobileNetV3 search space, MOEA-BUS achieves a 0.75% advantage in classification accuracy, while the obtained MOEA-BUS-XL has a smaller number of parameters.

## II. Ablation study of surrogate model

The surrogate model is utilized in this paper to rapidly filter 60,000 architectures, thus its prediction accuracy is crucial for the results of this experiment. To exclude influences from the search process, we design an experiment focused specifically on the surrogate model. The experimental results are presented in Fig. 1, where each subplot has the horizontal axis repre-

This work was supported by the National Natural Science Foundation of China (NO. 62376127, NO. 61876089, NO. 61876185), the Guangdong Basic and Applied Basic Research Foundation (No. 2024B1515020019), and the Natural Science Foundation of Shandong Province (NO. ZR2023ZD06). *(Corresponding author: Yu Xue.)*

Yu Xue, Pengcheng Jiang and Chenchen Zhu are with the School of Software, Nanjing University of Information Science and Technology, Nanjing 210044, China (e-mails: xueyu@nuist.edu.cn; pcjiang@nuist.edu.cn; 202212490283@nuist.edu.cn).

Yong Zhang is with the School of Information and Control Engineering, China University of Mining and Technology, Xuzhou 221008, China (e-mail: yongzh401@cumt.edu.cn).

Ran Cheng is with the Department of Data Science and Artificial Intelligence, and the Department of Computing, The Hong Kong Polytechnic University, Hong Kong SAR, China, and also with The Hong Kong Polytechnic University Shenzhen Research Institute, Shenzhen, China (e-mail: ranchengcn@gmail.com).

Kaizhou Gao is with the Macau Institute of Systems Engineering, Macau University of Science and Technology, Taipa 999078, Macao SAR, China (e-mail: kzgao@must.edu.mo).

Dunwei Gong is with the College of Automation and Electronic Engineering, Qingdao University of Science and Technology, Qingdao 266061, Shandong, China (e-mail: dwgong@qust.edu.cn).

TABLE I: Comparison on the CIFAR-100 dataset. This table compares the classification accuracy, computational complexity (MAdds), and search cost with other state-of-the-art NAS methods on the CIFAR-100 dataset.

| **Architecture** | **Accuracy (%)** | **MAdds (M)** | **Params (M)** | **Search Cost (GPU Days)** | **Search Method** | **Year** |
|---|---|---|---|---|---|---|
| MobileNetV2 [1] | 80.8 | 300 | 3.4 | - | manual | 2018 |
| EfficientNet-B0 [2] | **88.1** | 400 | 4.0 | - | manual | 2019 |
| NASNet-A Large [3] | 86.7 | 12031 | - | 1800 | RL | 2018 |
| NASNet-A mobile [3] | 83.9 | 600 | - | 1800 | RL | 2018 |
| DBNAS-B [4] | 84.54 | - | 3.3 | - | RL | 2025 |
| MixNet-M [5] | 86.11 | 200 | 2.1 | - | GD | 2019 |
| PC-DARTS [6] | 83.1 | - | 3.6 | 0.3 | GD | 2019 |
| EoiNAS [7] | 82.7 | - | 3.4 | 0.6 | GD | 2022 |
| GENAS [8] | 83.14 | 504 | 3.53 | 0.26 | GD | 2024 |
| SWD-NAS [9] | 83.87 | - | 3.56 | 0.13 | GD | 2024 |
| DBNAS-A [4] | 85.18 | - | 2.5 | - | GD | 2025 |
| DBNAS-C [4] | 84.74 | - | 3.0 | - | GD | 2025 |
| FX-DARTS [10] | 77.93±0.08 | 195 | 1.26 | 0.11 | GD | 2025 |
| NSGA-Net [11] | 80.17 | - | 11.6 | 8 | EA | 2019 |
| MUXNet-M [12] | 86.11 | 200 | 2.1 | 11 | EA | 2020 |
| FairNAS-A [13] | 87.3 | 391 | - | 12 | EA | 2021 |
| FairNAS-B [13] | 87 | 348 | - | 12 | EA | 2021 |
| FairNAS-C [13] | 86.7 | 324 | - | 12 | EA | 2021 |
| ZenNet [14] | 84.4 | 487 | | 0.5 | EA | 2021 |
| MPAE-A [15] | 82.74 | - | 4.2 | 0.3 | EA | 2024 |
| MPAE-B [15] | 83.45 | - | 4.8 | 0.3 | EA | 2024 |
| MPAE-C [15] | 84.12 | - | 5.2 | 0.3 | EA | 2024 |
| MPE-NAS [16] | 80.41 | - | 6.6 | 0.81 | EA | 2024 |
| PEPNAS [17] | 83.95 | - | 4.34 | 0.85 | EA | 2024 |
| SPNAS [18] | 87.26 | - | 6.7 | 1.6 | EA | 2025 |
| MOEA-BUS-S | 86.71±0.03 | 198 | 4.19 | 1.2 | EA | - |
| MOEA-BUS-M | 87.20±0.03 | 273 | 4.77 | 1.2 | EA | - |
| MOEA-BUS-L | 87.53±0.04 | 458 | 6.24 | 1.2 | EA | - |
| MOEA-BUS-XL | 88.01±0.03 | 657 | 6.30 | 1.2 | EA | - |

TABLE II: Time cost of different machine learning model as the surrogate with regression/pairwise surrogate mode.

| Surrogate mode | Machine learning model | Ktau | Training time (seconds) | Prediction time (seconds) |
|---|---|---|---|---|
| Regression | Random forest | 0.6807 | 0.33 | 0.02 |
| | Support vector machine | 0.7492 | 0.003 | 0.009 |
| | Multilayer perceptron | 0.6276 | 34.16 | 0.02 |
| | AdaBoost | 0.7228 | 0.033 | 0.003 |
| Pairwise | Random forest | 0.6991 | 7.78 | 4.14 |
| | Support vector machine | **0.7721** | 48.33 | 166.39 |
| | Multilayer perceptron | 0.6524 | 657 | 2.43 |
| | AdaBoost | 0.7371 | 4.93 | 0.97 |

senting the real ranking of 1000 architectures and the vertical axis representing the predicted ranking. The dots closer to the diagonal line indicate better prediction performance. We collect the execution processes from all our previous experiments on the ImageNet dataset, obtaining historical information for approximately 7,000 architectures in total. We perform sampling among these architectures to simulate the impact of different sampling methods on the surrogate model. We sample 1,300 architectures from these candidates, where 300 architectures are used for training the surrogate model and 1000 architectures are employed to evaluate its performance. The results using random sampling are plotted in Figures 1a - 1h, while the results using uniform sampling are depicted in Figures 1i - 1p. We select four commonly used machine learning models as base models, including random forest (RF), support vector machine (SVM), multilayer perceptron (MLP), and AdaBoost. In this paper, proposed surrogate model employs pairwise prediction methods, therefore in our additional experiments, we compare the performance of pairwise prediction with regression prediction. In each subplot title, "-R" indicates regression prediction and "-C" indicates pairwise prediction. Additionally, in the parentheses of each subplot title, "$\mathbf{R}$" represents random sampling, "$\mathbf{U}$" represents uniform sampling, and the floating-point numbers represent the Kendall's tau correlation coefficient (Ktau) calculated between predicted rankings and real rankings. According to Fig. 1, we can intuitively observe the impact of different surrogate patterns (regression prediction and pairwise comparison relationship prediction), initialization methods, and base machine learning models on surrogate performance. It can also be observed that both uniform sampling and pairwise prediction can stably enhance the prediction performance of the surrogate model with each base machine learning model. For example, according to Figures 1f and 1n, the SVM method used in this paper can achieve a 0.07 Ktau improvement when employing the proposed uniform sampling initialization method. According to Figures 1m - 1p, using different base machine learning models also affects surrogate performance, and the employed SVM can achieve at least a 0.035 Ktau improvement compared to other models. Our results demonstrate that the surrogate model employed in the methodology effectively adapts to uniform sampling, enabling accurate performance prediction

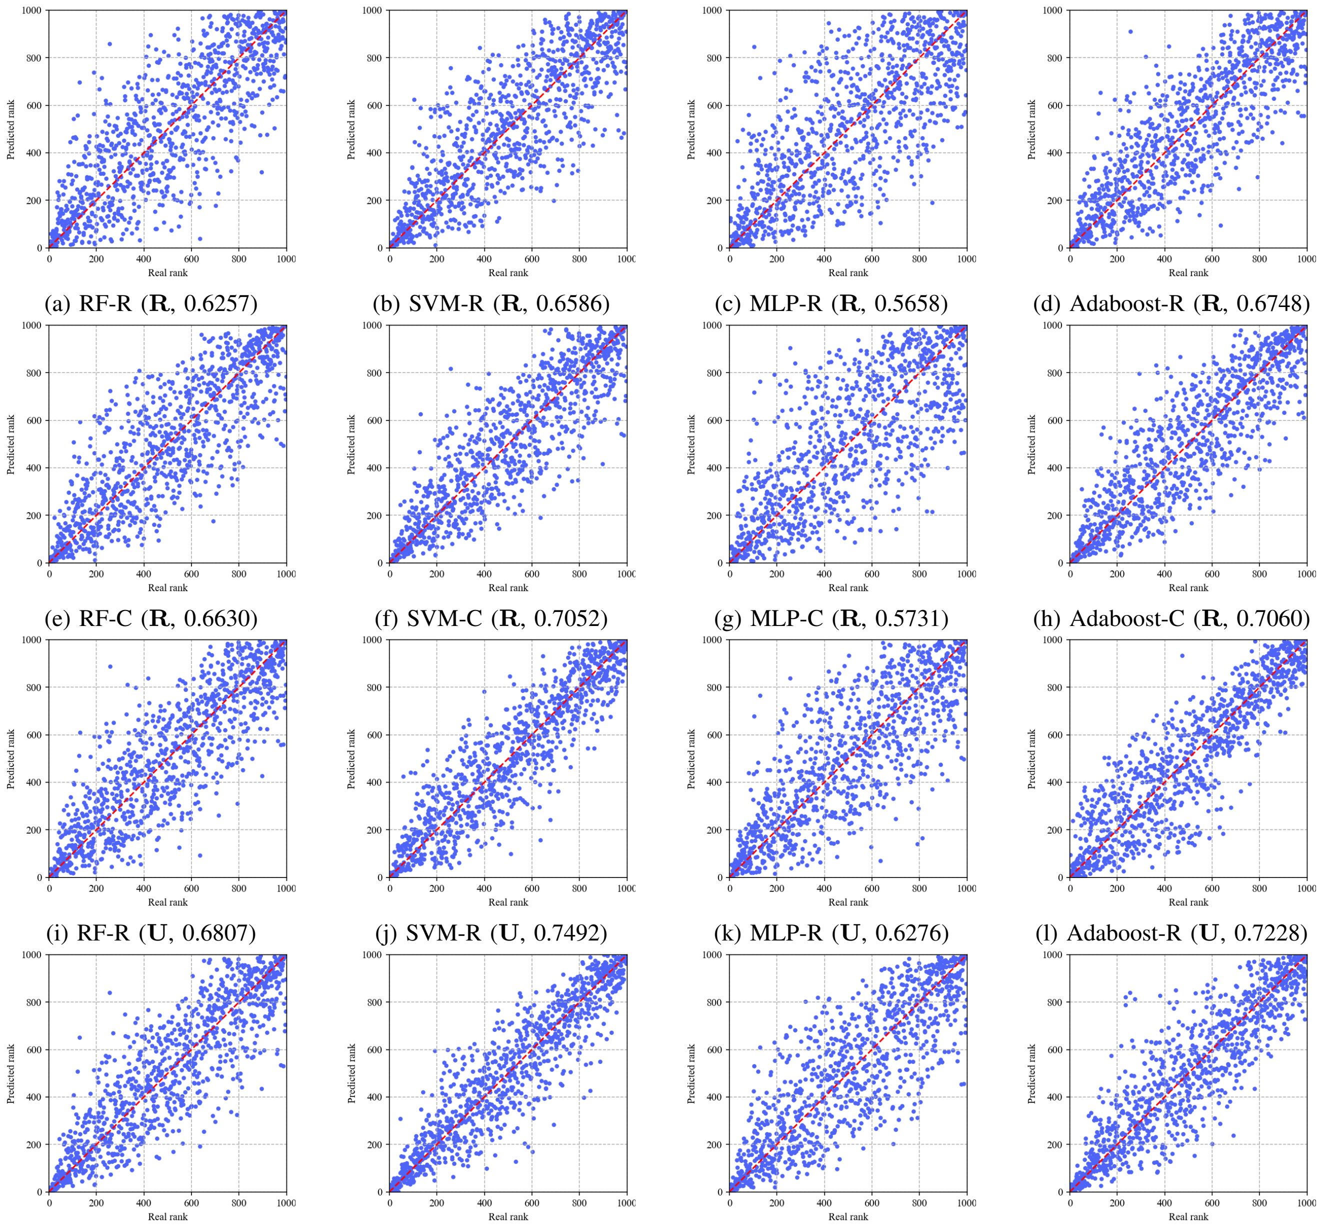


(a) RF-R (**R**, 0.6257) (b) SVM-R (**R**, 0.6586) (c) MLP-R (**R**, 0.5658) (d) Adaboost-R (**R**, 0.6748)

(e) RF-C (**R**, 0.6630) (f) SVM-C (**R**, 0.7052) (g) MLP-C (**R**, 0.5731) (h) Adaboost-C (**R**, 0.7060)

(i) RF-R (**U**, 0.6807) (j) SVM-R (**U**, 0.7492) (k) MLP-R (**U**, 0.6276) (l) Adaboost-R (**U**, 0.7228)

(m) RF-C (**U**, 0.6991) (n) SVM-C (**U**, 0.7721) (o) MLP-C (**U**, 0.6524) (p) Adaboost-C (**U**, 0.7371)

Fig. 1: Ablation study on surrogate model prediction performance using four different machine learning models, including the SVM adopted in this paper.

of candidate architectures.

## III. Study on Surrogate Time Cost

To further analyze the time consumption of the surrogate process, we conduct statistics on the time consumption for training surrogate models and predicting architecture performance in the experiments from Section II. We collect the time consumption for each base machine learning model under both regression prediction and pairwise comparison relation prediction modes, and present the results in Table II. Although the proposed method incurs the highest time consumption, the training time remains within 1 minute, and the time overhead for pairwise comparison relation prediction on 1,000 architectures is within 3 minutes. Since the number of individuals that need to be evaluated simultaneously in each iteration of the search process does not exceed 150, the time overhead will be significantly reduced. Therefore, we are confident that this is acceptable for neural architecture search (NAS) problems.

## References

[1] M. Sandler, A. Howard, M. Zhu, A. Zhmoginov, and L.-C. Chen, "MobileNetV2: Inverted residuals and linear bottlenecks," in *Proceedings of the IEEE Conference on Computer Vision and Pattern Recognition*, 2018, pp. 4510–4520.

[2] M. Tan and Q. Le, "EfficientNet: Rethinking model scaling for convolutional neural networks," in *Proceedings of the 36th International Conference on Machine Learning*, 2019, pp. 6105–6114.

[3] B. Zoph, V. Vasudevan, J. Shlens, and Q. V. Le, "Learning transferable architectures for scalable image recognition," in *Proceedings of the IEEE/CVF Conference on Computer Vision and Pattern Recognition*, 2018, pp. 8697–8710.

[4] A. Yang, Y. Liu, C. Li, and Q. Ren, "Deeply supervised block-wise neural architecture search," *IEEE Transactions on Neural Networks and Learning Systems*, vol. 36, no. 2, pp. 2451–2464, 2025.

[5] M. Tan and Q. V. Le, "MixConv: Mixed depthwise convolutional kernels," in *British Machine Vision Conference*, 2019, p. 74.

[6] Y. Xu, L. Xie, X. Zhang, X. Chen, G.-J. Qi, Q. Tian, and H. Xiong, "PC-DARTS: Partial channel connections for memory-efficient architecture search," in *International Conference on Learning Representations*, 2019.

[7] Y. Zhou, X. Xie, and S.-Y. Kung, "Exploiting operation importance for differentiable neural architecture search," *IEEE Transactions on Neural Networks and Learning Systems*, vol. 33, no. 11, pp. 6235–6248, 2022.

[8] Y. Xue, X. Han, F. Neri, J. Qin, and D. Pelusi, "A gradient-guided evolutionary neural architecture search," *IEEE Transactions on Neural Networks and Learning Systems*, vol. 36, no. 3, pp. 4345–4357, 2025.

[9] Y. Xue, X. Han, and Z. Wang, "Self-adaptive weight based on dual-attention for differentiable neural architecture search," *IEEE Transactions on Industrial Informatics*, vol. 20, no. 4, pp. 6394–6403, 2024.

[10] X. Rao, B. Zhao, D. Liu, and C. Alippi, "FX-DARTS: Designing topology-unconstrained architectures with differentiable architecture search and entropy-based super-network shrinking," *IEEE Transactions on Neural Networks and Learning Systems*, vol. 36, no. 10, pp. 19 356–19 369, 2025.

[11] Z. Lu, I. Whalen, V. Boddeti, Y. Dhebar, K. Deb, E. Goodman, and W. Banzhaf, "NSGA-Net: Neural architecture search using multi-objective genetic algorithm," in *Proceedings of the Genetic and Evolutionary Computation Conference*, 2019, pp. 419–427.

[12] Z. Lu, K. Deb, and V. N. Boddeti, "MUXConv: Information multiplexing in convolutional neural networks," in *Proceedings of the IEEE/CVF Conference on Computer Vision and Pattern Recognition*, 2020, pp. 12 044–12 053.

[13] X. Chu, B. Zhang, and R. Xu, "FairNAS: Rethinking evaluation fairness of weight sharing neural architecture search," in *Proceedings of the IEEE/CVF International Conference on Computer Vision*, 2021, pp. 12 239–12 248.

[14] M. Lin, P. Wang, Z. Sun, H. Chen, X. Sun, Q. Qian, H. Li, and R. Jin, "Zen-NAS: A zero-shot NAS for high-performance image recognition," in *Proceedings of the IEEE/CVF International Conference on Computer Vision*, 2021, pp. 337–346.

[15] J. Zou, H. Chu, Y. Xia, J. Xu, Y. Liu, and Z. Hou, "Multiple population alternate evolution neural architecture search," in *2025 International Joint Conference on Neural Networks (IJCNN)*, 2025, pp. 1–9.

[16] C. Song, Y. Ma, Y. Xu, and H. Chen, "Multi-population evolutionary neural architecture search with stacked generalization," *Neurocomputing*, vol. 587, p. 127664, 2024.

[17] Y. Xue, J. Zha, D. Pelusi, P. Chen, T. Luo, L. Zhen, Y. Wang, and M. Wahib, "Neural architecture search with progressive evaluation and sub-population preservation," *IEEE Transactions on Evolutionary Computation*, vol. 29, no. 5, pp. 1678–1691, 2025.

[18] P. Jiang, Y. Xue, and F. Neri, "Score predictor-assisted evolutionary neural architecture search," *IEEE Transactions on Emerging Topics in Computational Intelligence*, 2025, DOI: 10.1109/TETCI.2025.3526179.
